# Supplementary material for: Scale-Free Networks beyond Power-Law Degree Distribution
Source: arXiv:2310.08110 source file (2023-10-21)
Supplement: Supplementary file 1 [file suppl.pdf]

# Supplementary Information:
# Scale-Free Networks beyond Power-Law Degree Distribution

Xiangyi Meng[1,2] and Bin Zhou[3,*]

[1]*Network Science Institute and Department of Physics, Northeastern University, Boston, Massachusetts 02115, USA*
[2]*Department of Physics and Astronomy, Northwestern University, Evanston, Illinois 60208, USA*
[3]*School of Management Science and Engineering, Nanjing University of Information Science and Technology, Nanjing, 210044, China*

## Contents

**1 Derive the degree–degree distance distribution from the joint probability distribution** **2**

**2 Preferential attachment of internal links** **3**

**3 Fitness with threshold** **5**

**4 The Erdős–Rényi model** **7**

## 1 Derive the degree–degree distance distribution from the joint probability distribution

The degree–degree distance[1],

$$\eta = \exp\left|\ln k_i - \ln k_j\right|, \tag{1}$$

is defined for every link $i \leftrightarrow j$ that connects two nodes $i$ and $j$. Alternatively, we can write the degree–degree distance as $\eta = \max\{k_i/k_j, k_j/k_i\}$, namely, the ratio between the larger degree and the smaller degree of the two nodes that the link $i \leftrightarrow j$ connects. Therefore, the cumulative probability distribution of $\eta$ is given by

$$\mathcal{P}(H \le \eta) = \mathcal{P}(Y/\eta < X \le Y\eta) = \int_{\max\{y/\eta, k_{\min}\}}^{\eta y} dx \int_{k_{\min}}^{\infty} dy\ \mathcal{P}\left(\{x,y\}|i \leftrightarrow j\right), \tag{2}$$

where the composite random variable $H$ is given by $\ln H = |\ln X - \ln Y|$, and the conditional joint probability $\mathcal{P}\left(\{k_i,k_j\}|i \leftrightarrow j\right)$ is defined as the probability of sequentially selecting two nodes $i$ and $j$ that have degrees $k_i, k_j \in [k_{\min}, \infty)$, respectively, conditioned on $i$ and $j$ being connected. Note that the conditional joint probability is symmetric, i.e., $\mathcal{P}\left(\{k_i,k_j\}|i \leftrightarrow j\right)$=$\mathcal{P}\left(\{k_j,k_i\}|i \leftrightarrow j\right)$. Given a tuple $(x,y)$, the sum $\mathcal{P}\left(\{x,y\}|i \leftrightarrow j\right) + \mathcal{P}\left(\{y,x\}|i \leftrightarrow j\right)$ denotes the fraction of links that connect two nodes of degree $x$ and degree $y$.

By Eq. (2), the probability density distribution of $\eta$ can be written as

$$\begin{aligned} g(\eta) &= \frac{d\mathcal{P}(H \le \eta)}{d\eta} = \int_{k_{\min}}^{\infty} \mathcal{P}(\{\eta y, y\}|i \leftrightarrow j) y dy + \int_{\eta k_{\min}}^{\infty} \mathcal{P}(\{y/\eta, y\}|i \leftrightarrow j)\frac{y}{\eta^2} dy \\ &= \int_{k_{\min}}^{\infty} 2\mathcal{P}(\{\eta y, y\}|i \leftrightarrow j) y dy. \end{aligned} \tag{3}$$

Equation (3) allows us to calculate the degree–degree distance distribution $g(\eta)$ from the conditional joint probability $\mathcal{P}\left(\{k_i,k_j\}|i \leftrightarrow j\right)$. For example, the conditional joint probability of the Barabási-Albert (BA) model[2] is given by

$$\mathcal{P}(\{k_i,k_j\}|i \leftrightarrow j) \simeq \frac{k_{\min}\left(k_{\min}+1\right)}{k_i\left(k_i+1\right)k_j\left(k_j+1\right)}\left[1 - \frac{\binom{2k_{\min}+2}{k_{\min}+1}\binom{k_i+k_j-2k_{\min}}{k_j-k_{\min}}}{\binom{k_i+k_j+2}{k_j+1}}\right] \tag{4}$$

(which differs from the known result[3] by a factor of 2, because here we define nodes $i$ and $j$ to be *sequentially* selected). Thus, by Eq. (3), we have

$$g(\eta) \simeq 2\left(k_{\min}+1\right)\left(1 + k_{\min}\ln\frac{k_{\min}}{1+k_{\min}}\right)\eta^{-2} + \cdots. \tag{5}$$

## 2 Preferential attachment of internal links

In the "no-growth" model, the probability of attaching a link to a node of degree $k$ at time step $T$ is given by

$$2\left(k+b\right)/\sum_{i=1}^{N}\left(k_i+b\right)=2\left(k+b\right)/\left(2T+bN\right), \tag{6}$$

where the factor of 2 accounts for the fact that *two* nodes are connected at each time step. This allows us to write down the rate equation for $f(T,k)$, the probability that a node has degree $k$ at time step $T$, as

$$f(T+1,k)=\left[\frac{2\left(k-1+b\right)}{2T+bN}\right]f(T,k-1)+\left[1-\frac{2\left(k+b\right)}{2T+bN}\right]f(T,k), \tag{7}$$

where the first term on the right-hand side denotes the probability that a node of degree $k-1$ is selected at time step $T$, and the second term denotes the probability that a node of degree $k$ is *not* selected at time step $T$. Since Eq. (7) is Markovian, it can be written as a differential equation in the continuous limit, namely,

$$T'\frac{\partial f}{\partial T'}=-\frac{\partial}{\partial k'}\left(k'f\right), \tag{8}$$

where $T'=T+bN/2$ and $k'=k+b$.

When $b$ is small, we assume that the solution of Eq. (8) approximately follows a Gamma distribution,

$$f(T,k)=e^{-B(T)k}k^{A-1}B(T)^A/\Gamma(A). \tag{9}$$

To fix the parameters $A$ and $B(T)$, note that at the boundary $k=0$, we have

$$\begin{aligned} f(T,0) &= \prod_{t=1}^{T}\left[1-\frac{2b}{2\left(t-1\right)+bN}\right]=\frac{\Gamma\left(\frac{bN}{2}\right)\Gamma\left(T+\frac{bN-b}{2}\right)}{\Gamma(T+\frac{bN}{2})\Gamma\left(\frac{bN-b}{2}\right)}=\left(\frac{bN}{2}-b\right)_T/\left(\frac{bN}{2}\right)_T \\ &\simeq \left(\frac{bN}{2T}\right)^b+O(N^{b-1}), \end{aligned} \tag{10}$$

where $(x)_n=\Gamma(x+n)/\Gamma(x)$ is the Pochhammer symbol. Recall that the general solution of Eq. (8) for small $b$ is $f(T,k)=T^{-1}\mathcal{F}(k/T)$, where $\mathcal{F}(x)$ is an arbitrary function. This allows us to match the terms involving $k$ and $T$ in Eqs. (9) and (10), finding that $A=b$ and $B(T)=bN/\left(2T\right)$.

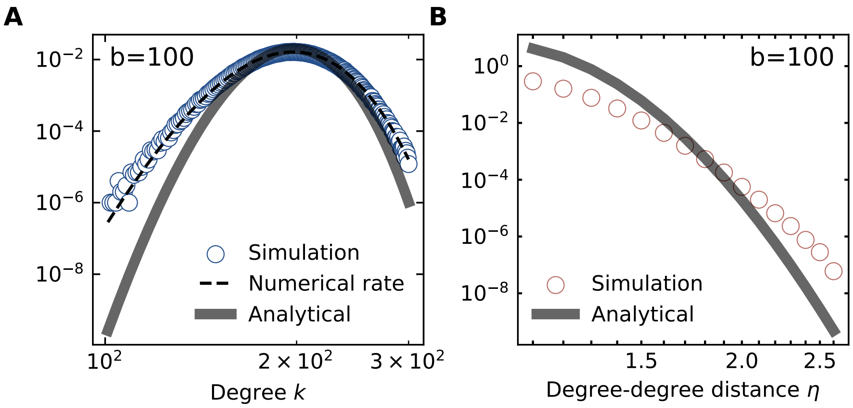


Figure 1: (a,b) Distributions of (a) $k$ and (b) $\eta$ for the "no-growth" model. The model simulation results (circle) are given by the average of $10^2$ runs on $N = 10^4$ nodes and $T = 10^6$ links; the analytical solutions are derived from the Gamma-distribution ansatz [Eq. (9)]; and the numerical solution is derived directly from the rate equation [Eq. (7)].

When $b$ is large, the Gamma-distribution ansatz [Eq. (9)] is no longer valid, but the numerical solution of the rate equation [Eq. (7)] still matches the simulation result of DD (Fig. 1).

*The Facebook network.*—The empirical DD and DDDD of the Facebook network [4] were obtained using the *log binning* approach. Ten log bins were assigned over the full range of $k$ and $\eta$, respectively. To fit the empirical DD and DDDD, we first ran a linear fit of the empirical DDDD on the log-log plot, finding that the power-law exponent was given by $2 + b \approx 2.41$. This allowed us to fix $b$ as $0.41$. Then, the DD and the DDDD of the no-growth model were plotted under $b = 0.41$, $N = 10^6$, and $T = 10^8$, for which $R^2$ was calculated against the empirical DD and DDDD.

## 3 Fitness with threshold

In the "hard-threshold" model, the conditional probability that a node has degree $k$ given fitness $\omega_i$ is a binomial distribution, $\mathcal{P}(k|\omega_i) \simeq \binom{N}{k} p(\omega_i)^k \left(1 - p(\omega_i)\right)^{N-k}$, where $p(\omega_i) = \max\{1 - (z - \omega_i)/\omega_{\max}, 0\}$. It can be approximated as a Gaussian distribution,

$$\mathcal{P}(k|\omega_i) \simeq \frac{1}{\sqrt{2\pi}\sigma_i} e^{-\frac{(k-\mu_i)^2}{2\sigma_i^2}}, \tag{11}$$

where $\mu_i = Np(\omega_i)$ and $\sigma_i^2 = Np(\omega_i)\left(1 - p(\omega_i)\right)$ are the mean and variance, respectively. Given $\mu_i^2 = O(N^2)$ and $\sigma_i^2 = O(N)$, in the large $N$ limit, the Gaussian distribution can be approximated as a delta function, i.e., $\mathcal{P}(k|\omega_i) \simeq \delta(k - \mu_i)$. Hence, we have

$$f(k) = \int_0^{\omega_{\max}} \mathcal{P}(k|\omega_i)\rho(\omega_i) d\omega_i \simeq \int_{z-\omega_{\max}}^{\omega_{\max}} \frac{\delta(k-\mu_i) d\omega_i}{2\omega_{\max} - z} \simeq \frac{N^{-1}}{2 - z/\omega_{\max}} + O(N^{-2}). \tag{12}$$

Note that in the second step of Eq. (12), the lower limit of the integration becomes $z - \omega_{\max}$. This is because the delta-function approximation works only if $\omega_i > z - \omega_{\max}$; otherwise one always has $p(\omega_i) = 0$. As a result, $\rho(\omega_i) = \omega_{\max}^{-1}$ is changed to $\rho(\omega_i) = (2\omega_{\max} - z)^{-1}$ for proper normalization of $f(k)$. In the third step, the scaling property $\delta(\alpha x) = |\alpha|^{-1}\delta(x)$ of the delta function is used.

To solve the DDDD, from Eq. (11) we have

$$\begin{aligned}\mathcal{P}(\eta k|\omega_i)\mathcal{P}(k|\omega_j) &\simeq \frac{1}{\sqrt{2\pi}\sqrt{\sigma_i^2 + \eta^2\sigma_j^2}} \exp\left[-\frac{(\mu_i - \eta\mu_j)^2}{2\left(\sigma_i^2 + \eta^2\sigma_j^2\right)}\right] \frac{1}{\sqrt{2\pi}\sqrt{\frac{\sigma_i^2\sigma_j^2}{\sigma_i^2+\eta^2\sigma_j^2}}} \exp\left[-\frac{\left(k - \frac{\eta\mu_i\sigma_j^2 + \mu_j\sigma_i^2}{\sigma_i^2+\eta^2\sigma_j^2}\right)^2}{2\left(\frac{\sigma_i^2\sigma_j^2}{\sigma_i^2+\eta^2\sigma_j^2}\right)}\right] \\ &\simeq \frac{1}{\sqrt{2\pi}\sqrt{\sigma_i^2 + \eta^2\sigma_j^2}} \exp\left[-\frac{(\mu_i - \eta\mu_j)^2}{2\left(\sigma_i^2 + \eta^2\sigma_j^2\right)}\right] \delta\left(k - \frac{\eta\mu_i\sigma_j^2 + \mu_j\sigma_i^2}{\sigma_i^2 + \eta^2\sigma_j^2}\right),\end{aligned} \tag{13}$$

where $\mathcal{P}(\eta k|\omega_i)$ and $\mathcal{P}(k|\omega_j)$ are recombined into two Gaussian distributions, one depending on $k$ (which is further approximated as a delta function) while the other one not. Hence, the DDDD is given by

$$\begin{aligned} g(\eta) &= \int_1^\infty 2kdk \int_0^{\omega_{\max}} d\omega_i \int_0^{\omega_{\max}} d\omega_j \mathcal{P}(\eta k|\omega_i)\mathcal{P}(k|\omega_j)\mathcal{P}\left(\{\omega_i, \omega_j\}|i \leftrightarrow j\right) \\ &= \frac{\omega_{\max}^{-2}N^2}{2T} \int_1^\infty 2kdk \int_{z-\omega_{\max}}^{\omega_{\max}} d\omega_i \int_{z-\omega_i}^{\omega_{\max}} d\omega_j \mathcal{P}(\eta k|\omega_i)\mathcal{P}(k|\omega_j) \\ &\simeq \frac{\omega_{\max}^{-2}N^2}{2T} \int_{z-\omega_{\max}}^{\omega_{\max}} d\omega_i \int_{z-\omega_i}^{\omega_{\max}} d\omega_j \frac{2\left(\eta\mu_i\sigma_j^2 + \mu_j\sigma_i^2\right)}{\sigma_i^2 + \eta^2\sigma_j^2} \frac{1}{\sqrt{2\pi}\sqrt{\sigma_i^2 + \eta^2\sigma_j^2}} \exp\left[-\frac{(\mu_i - \eta\mu_j)^2}{2\left(\sigma_i^2 + \eta^2\sigma_j^2\right)}\right] \\ &\simeq \frac{\omega_{\max}^{-2}N^2}{2T} \int_{(\eta\omega_{\max} - \omega_{\max} + z)/(\eta+1)}^{\omega_{\max}} d\omega_i \, 2\eta^{-5/2}(\omega_i + \omega_{\max} - z)\sqrt{(\eta - 1) + 2\left(z - \omega_i\right)/\omega_{\max}} \\ &\simeq \frac{N^2(2 - z/\omega_{\max})^2\left(2\eta + 1\right)}{2T\eta^2\left(\eta + 1\right)^2} + O(N^1), \end{aligned} \tag{14}$$

where in the second step the result $\mathcal{P}\left(\{\omega_i, \omega_j\}|i \leftrightarrow j\right) = \theta(\omega_i + \omega_j - z) \cdot \omega_{\max}^{-2} N^2 T^{-1}/2$ is used (derived in the main text of the paper); in the second last step the integration on $\omega_j$ is approximated using the Laplace's method around the peak $\mu_j \simeq \mu_i/\eta$, or $\omega_j \simeq \omega_i/\eta + (z - \omega_{\max})(1 - 1/\eta)$; and the lower limit of the integration on $\omega_i$ is adjusted accordingly to ensure that $\omega_i + \omega_j \simeq \omega_i + \omega_i/\eta + (z - \omega_{\max})(1 - 1/\eta) > z$.

*The WorldCity network.*—Again, the empirical DD and DDDD of the WorldCity network [5] were obtained using the log binning approach. Ten log bins were assigned over the full range of $k$ and $\eta$, respectively. To fit the empirical DD and DDDD, we first ran a flat fit of the empirical DD on the log-log plot, finding that the normalization coefficient was given by $N^{-1}/(2 - z/\omega_{\max}) \approx 0.048$. This allowed us to fix $z/\omega_{\max}$ as $1.95$. Then, the DD and the DDDD of the hard-threshold model were plotted under $z = 1.95\omega_{\max}$, $N = 415$, and $T = 7,518$, for which $R^2$ was calculated against the empirical DD and DDDD.

Technically, the parameters $N$, $T$, and $z/\omega_{\max}$ in Eq. (14) are not independent from each other. When $N$ is large, the density of links $2T/N^2$ converges to $\left(2 - z/\omega_{\max}\right)^2/2$. When fitting to the WorldCity network, however, it is worth noting that the network is bipartite, only containing connections between cities and firms [5], and therefore the number of possible connections is smaller than $N^2/2$. This results in an extra normalization constant in Eq. (14) that is absorbed into the degree of freedom of $z/\omega_{\max}$.

## 4 The Erdős–Rényi model

Similar to the calculation of the hard-threshold model, we approximate the DD of the Erdős–Rényi (ER) model[6] by a Gaussian distribution (by fixing the linking probability $p_0$),

$$f(k) \simeq \frac{1}{\sqrt{2\pi}\sigma} e^{-\frac{(k-\mu)^2}{2\sigma^2}}, \tag{15}$$

where $\mu = Np_0$ and $\sigma^2 = Np_0 (1 - p_0)$ are the mean and variance. The conditional joint probability

$$\mathcal{P}\left(\{k_i, k_j\} | i \leftrightarrow j\right) = \frac{k_i f(k_i)}{\mu} \frac{k_j f(k_j)}{\mu}$$

can be written as the product of two independent marginal distributions, $kf(k)/\mu$, denoting the probability of selecting a link that is connected to a node of degree $k$. The DDDD is thus given by

$$\begin{aligned} g(\eta) &= \int_1^\infty 2\mathcal{P}\left(\{\eta k, k\} | i \leftrightarrow j\right) k dk \\ &\simeq \frac{2\eta}{\mu^2} \int_1^\infty dk \frac{k^3}{\sqrt{2\pi}\sqrt{\sigma^2 + \eta^2\sigma^2}} \exp\left[-\frac{(\mu - \eta\mu)^2}{2\left(\sigma^2 + \eta^2\sigma^2\right)}\right] \delta\left(k - \frac{\eta\mu\sigma^2 + \mu\sigma^2}{\sigma^2 + \eta^2\sigma^2}\right) \\ &\simeq \left[\frac{2Np_0}{\pi(1 - p_0)}\right]^{1/2} \frac{\eta\left(\eta + 1\right)^3}{\left(\eta^2 + 1\right)^{7/2}} e^{-\frac{Np_0(\eta-1)^2}{2(1-p_0)(\eta^2+1)}}, \end{aligned} \tag{16}$$

where in the second step the combination of two Gaussian distributions [Eq. (13)] is once again used.

Note that Eq. (16) is only valid when taking $N \to \infty$ while fixing $p_0$. If, however, we take $p_0 \sim N^{-1}$ such that $Np_0$ is of order one, then $f(k)$ tends to a Poisson distribution. In that case, Eq. (16) is no longer valid and would incorrectly predict a power-law DDDD $g(\eta) \sim \eta^{-3}$, which is not observed in simulation (Fig. 2).

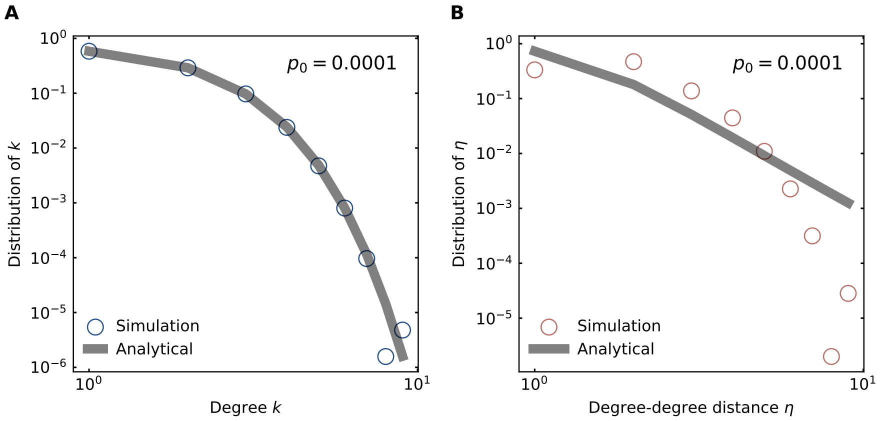


Figure 2: Distributions of (a) $k$ and (b) $\eta$ for the Erdős–Rényi model, given the linking probability $p_0 = N^{-1}$. The model simulation results (circle) are given by the average of $10^2$ runs on $N = 10^4$ nodes.

## References


1. Zhou, B., Meng, X. & Stanley, H. E. Power-law distribution of degree–degree distance: A better representation of the scale-free property of complex networks. *Proc. Natl. Acad. Sci.* **117**, 14812–14818 (2020).

2. Barabási, A.-L. & Albert, R. Emergence of scaling in random networks. *Science* **286**, 509–512 (1999).

3. Fotouhi, B. & Rabbat, M. G. Degree correlation in scale-free graphs. *Eur. Phys. J. B* **86**, 510 (2013).

4. Gjoka, M., Kurant, M., Butts, C. T. & Markopoulou, A. Walking in Facebook: A case study of unbiased sampling of OSNs. In *2010 Proceedings IEEE Infocom*, 1–9 (IEEE, 2010).

5. Taylor, P. & Derudder, B. *World city network: A global urban analysis* (Routledge, 2015).

6. Erdős, P. & Rényi, A. On random graphs. *Publ. Math. Debr.* **6**, 290–297 (1959).
